# Supplementary material for: Self-Assembly of Liquid Crystals in Nanoporous Solids for Adaptive Photonic Metamaterials
Source: arXiv:1911.10052 source file (2019-11-22)
Supplement: Supplementary file 1 [file Electronic_Supporting_Information.pdf]

# Electronic Supporting Information

## Self-Assembly of Liquid Crystals in Nanoporous Solids for Adaptive Photonic Metamaterials


Kathrin Sentker,[1] Arda Yildirim,[2] Milena Lippmann,[3] Arne W. Zantop,[4] Florian Bertram,[5] Tommy Hofmann,[6] Oliver H. Seeck,[3] Andriy V. Kityk,[7] Marco G. Mazza,[4] Andreas Schönhals,[2] and Patrick Huber[1,*]

[1] *Institute for Materials Physics and Technology, Hamburg University of Technology (TUHH), Eißendorferstr. 42, D-21073 Hamburg, Germany*
[2] *Bundesanstalt für Materialforschung und -prüfung (BAM), Unter den Eichen 87, D-12205 Berlin, Germany*
[3] *DESY Photon Science, Notkestraße 85, D-22607 Hamburg, Germany*
[4] *Max-Planck-Institute for Dynamics and Self-Organization, Am Faßberg 17, D-37077 Göttingen, Germany*
[5] *Deutsches Elektronen-Synchrotron DESY, Notkestrasse 85, D-22607 Hamburg, Germany, Notkestraße 85, D-22607 Hamburg, Germany*
[6] *Helmholtz-Zentrum für Materialien und Energie, Hahn-Meitner-Platz 1, D-14109 Berlin, Germany*
[7] *Faculty of Electrical Engineering, Czestochowa University of Technology, Al. Armii Krajowej 17, P-42-200 Czestochowa, Poland*



(Dated: September 26, 2019)



* patrick.huber@tuhh.de

## NANOPOROUS MATERIALS

| Producer | Diameter $d$ (nm) | Porosity $P$ (%) | Thickness $t$ ($\mu$m) |
|---|---|---|---|
| SM | 16.7 ± 0.6 | 16 ± 1 | 108 |
| IR | 17.8 ± 1.75 | 19.35 ± 1.55 | 101 |
| OS | 24.3 ± 1.2 | 17.9 ± 0 | 101 |
| SM | 25.3 ± 0.2 | 28.8 ± 1 | 103 |
| SM | 34.2 ± 0.2 | 44.0 ± 0 | 85 |
| SM | 37.8 ± 0.7 | 15.8 ± 0.7 | 106 |
| SM | 47.3 ± 0.2 | 21.5 ± 0 | 79 |
| SM | 73 ± 3 | 36.5 ± 1.6 | 106 |
| IR | 86 ± 9 | 7.6 ± 0.6 | 101 |
| SM | 161 ± 10 | 13.8 ± 1.6 | 110 |

TABLE I. Pore diameter and porosities of AAO membranes as determined by $N_2$ sorption isotherms along with the membrane thicknesses. Producer are SmartMembranes GmbH (SM), InRedox LLC (IR) and the research group of M. Steinhart at University of Osnabrück (OS).

## OPTICAL RETARDATION EXPERIMENT

To determine the temperature dependent strength of the birefringence of a sample a measurement setup utilizing modulation spectroscopy is used as illustrated in Fig. S1(a). The setup, similar to that described in Ref. [1, 2], consists of a He-Ne-laser ($\lambda = 632.8\,\mathrm{nm}$) emitting linearly polarized light. After being linearly polarized at 45° to the direction of propagation by a polarizer the light passes through an optical photoelastic modulator (PEM). The PEM exhibits a time dependent birefringence due to the photoelastic effect

$$\Delta n_{\mathrm{PEM}} = \Delta n_0 \sin(\Omega t). \tag{1}$$

This results in a temporal modulated retardation

$$\delta_0 = \Delta n_o d_{\mathrm{M}} \sin(\Omega t) \tag{2}$$

with thickness of optical slab $d_{\mathrm{M}}$, retardation amplitude $\delta_0 = \Delta n_0 d_{\mathrm{M}} = 0.383\lambda$ and resonant frequency of the optical element $\Omega = 50\,\mathrm{kHz}$. This transparent and optical isotropic element is resonantly exposed to mechanical stress by a quartz piezoelectric transducer. Is the optical element relaxed the 45° linearly polarized light passes through the PEM unchanged. If it is compressed or stretched it exhibits birefringence, so that either the horizontal or vertical component of the electromagnetic wave travels faster, leading to a phase difference called retardation. The retardation depends on the strength of the birefringence and hence on the strength of the applied stress, which oscillates at $\Omega = 50\,\mathrm{kHz}$. Due to the resulting time dependent phase difference the electromagnetic wave is either linearly, circular or elliptically polarized after passing the PEM. Also the rotation direction of the polarization vector changes from left to right handed or *vice versa* during one period. In addition to this time dependent birefringence the laser light exhibits the static, temperature dependent birefringence $\Delta_0$ of the sample. Afterwards, the light passes an analyzer, that is set crossed to the polarizer, and is focused on a photo diode. The photo diode is connected to two lock-in amplifiers and detects the intensity of the first and second harmonic contribution of the laser light.

Considering a static birefringent sample in between crossed polarizer/analyzer the emerging wave vector projected on the analyzer axis, see Supplementary Fig. S1(b), is given by

$$\begin{aligned} E &= \frac{\sqrt{2}}{2} E_0 \cos(45^\circ) \sin(\omega t) \\ &\quad - \frac{\sqrt{2}}{2} E_0 \cos(45^\circ) \sin(\omega t - \delta) \\ &= \frac{1}{2} E_0 [\sin(\omega t) - \sin(\omega t - \delta)]. \end{aligned} \tag{3}$$

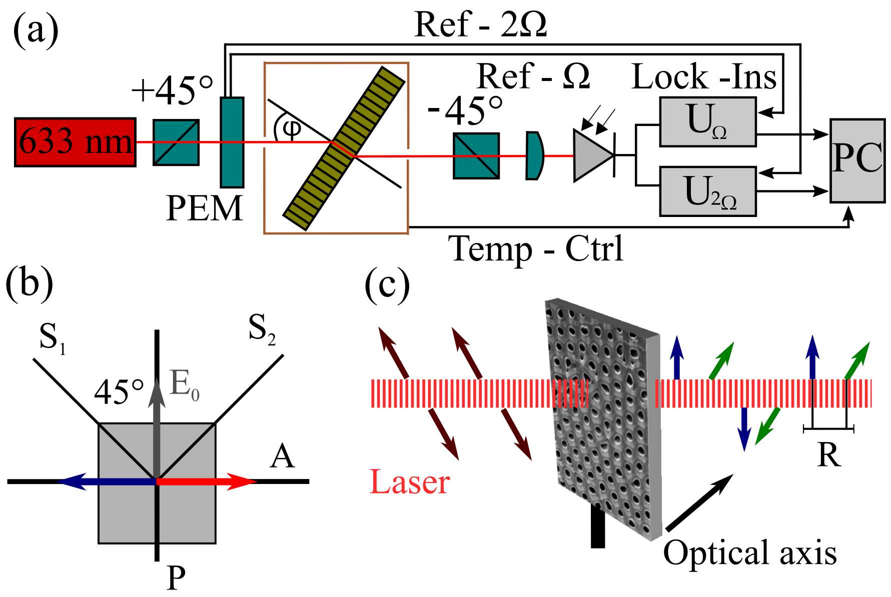


FIG. S1. (a) Schematic of optical retardation setup with (from left to right): He-Ne laser, polarizer (+45°), photoelastic modulator (PEM) with modulation frequency Ω, temperature cell, analyzer (-45°), lense, photodiode and lock-in amplifiers. (b) Simplified projection of polarization axes of polarizer and analyzer with respect to the anisotropic sample axes. (c) Alignment of sample approx. 45° with respect to the laser beam. Arrows show polarization of laser before and after passing the sample resulting in an optical retardation $R$.

with $\delta = \Delta n d$ and thickness $d$ of birefringent plate. Thereby the angle between incident laser light and anisotropic sample axis $S_1$ and $S_2$ is approx. 45° as illustrated in Supplementary Fig. S1(a) and (c). By taking the time average the intensity detected at the photo diode can be expressed by

$$I \sim \overline{E^2} \sim \overline{[\sin(\omega t) - \sin(\omega t - \delta)]^2} = 1 - \cos\delta. \tag{4}$$

Considering the time dependent birefringence induced by the PEM $\Delta_{\text{PEM}}$, see Eq. 1, and the temperature dependent birefringence of the sample $\Delta_x$ Eq. 4 can be expanded in Fourier series including Bessel functions $J_n$

$$I = 1 - \cos[\delta_x - \delta_0 \sin(\Omega t)] \tag{5}$$

$$= 1 - \cos(\delta_x)\cos[\delta_0 \sin(\Omega t)] + \sin(\delta_x)\sin[\delta_0 \sin(\Omega t)] \tag{6}$$

$$= 1 - \cos(\delta_x)\left(J_0(\delta_0) + 2\sum_{m=1}^{\infty} J_{2m}(\delta_0)\cos(2m\Omega t)\right) + \sin(\delta_x)\left(2\sum_{m=0}^{\infty} J_{2m+1}(\delta_0)\sin[(2m+1)\Omega t]\right). \tag{7}$$

The modulation amplitude is chosen so that $J_0(\delta_0) = 0$. The total signal can then be resolved as ac components at Ω and 2Ω. The lock-in technique eliminates the time dependency, so that the dc components of the intensity of the first and second harmonics can be used to calculate the optical retardation $R$

$$I_\Omega \sim J_1(\delta_0) 2\sin(\delta_x) \; I_{2\Omega} \sim J_2(\delta_0) 2\cos(\delta_x) \tag{8}$$

$$\Rightarrow \frac{I_\Omega}{I_{2\Omega}} = \frac{J_1(\delta_0)}{J_2(\delta_0)}\tan(\delta_x) \tag{9}$$

$$\Leftrightarrow \delta_x = \arctan\left(\frac{U_\Omega \cdot J_2(\delta_0)}{U_{2\Omega} \cdot J_1(\delta_0)}\right) = R \tag{10}$$

The contributions of the Bessel functions are constants of the experimental setup; $J_2(\delta_0)/J_1(\delta_0) = 0.83$. Equation 10 is only defined for rotation angles in between 0° and 90°. The data of samples that rotate the light polarization more than 90° need to be recalculated according to that. When $R$ hits 0° or 90° the phase of either the 1st or 2nd harmonic, as adjusted by the lock-ins, experiences a 180° jump. By performing reference measurements these jumps can be calibrated. A sample of known birefringence, e.g. positive geometrical birefringence, is rotated starting from perpendicular incident of the laser beam with respect to the sample surface.

Depending on the phase values the retardation either increases or decreases. This calibration can then be applied to the temperature curve of the retardation. Depending on this the sample either shows positive or negative birefringence.

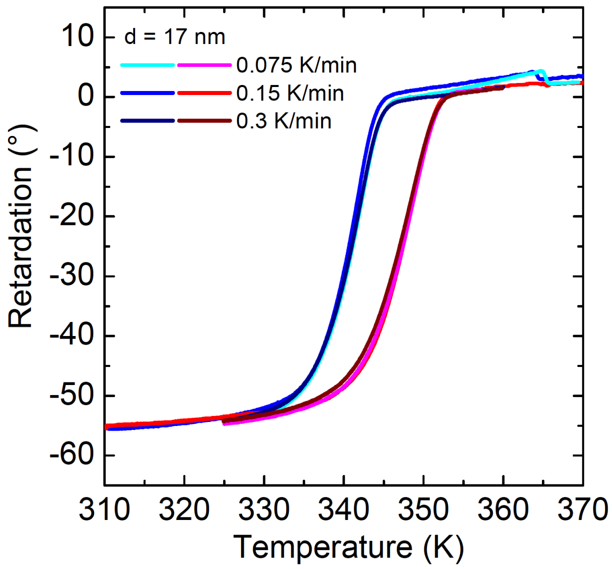


FIG. S2. Measured temperature-dependent optical retardation $R(T)$ for distinct heating/cooling rates as indicated in the figure for HAT6 in hydrophobic pores with 17 nm pore size. Data is normalized by the thickness and porosity of the corresponding AAO membrane, see Supplementary Tab. I.

## CALCULATION OF OPTICAL BIREFRINGENCE

For a tilted sample geometry as shown in Fig. S1 the optical retardation $R$ can be converted to the optical birefringence $\Delta n = n_e - n_o$ using Berek's equation

$$R = \frac{2\pi t(\overline{n} - \Delta n/3)}{\lambda}\{[1 - (\overline{n} + 2\Delta n/3)^{-2}\sin^2\theta]^{1/2} - [1 - (\overline{n} - \Delta n/3)^{-2}\sin^2\theta]^{1/2}\} \tag{11}$$

with sample thickness $t$, average refractive index $\overline{n} = (2n_o + n_e)/3$ and angle $\theta \approx 40°$ between laser beam and long pore axis. Considering an effective medium model for a AAO matrix (volume fraction $1 - P$) with cylindrical inclusions (volume fraction $P$), that represent the empty or completely filled channels, and assuming completely filled pores the average refractive index $\overline{n}$ can be estimated by solving the generalised Bruggemann equation [1]

$$P\frac{\varepsilon_{LC} - \varepsilon^{ef}_{\|,\perp}}{\varepsilon^{ef}_{\|,\perp} + L_{\|,\perp}(\varepsilon_{LC} - \varepsilon^{ef}_{j})} = (P-1)\frac{3(\varepsilon_{AAO} - \varepsilon^{ef}_{\|,\perp})}{2\varepsilon^{ef}_{\|,\perp} + \varepsilon_{AAO}}. \tag{12}$$

with porosity $P$, pore permittivity $\epsilon_{\|,\perp}$ parallel or perpendicular to the long pore axis and depolarisation factor $L_\| = 0$ and $L_\perp = 0.5$. The birefringence is then given by $\Delta n = \sqrt{\varepsilon_\|} - \sqrt{\varepsilon_\perp}$. The refractive index and hence permittivity of the DLC HAT6 and the empty AAO membrane are assumed to be $n_{LC} = \sqrt{\epsilon_{LC}} = 1.55$ and $n_{AAO} = \sqrt{\epsilon_{AAO}} = 1.76$.

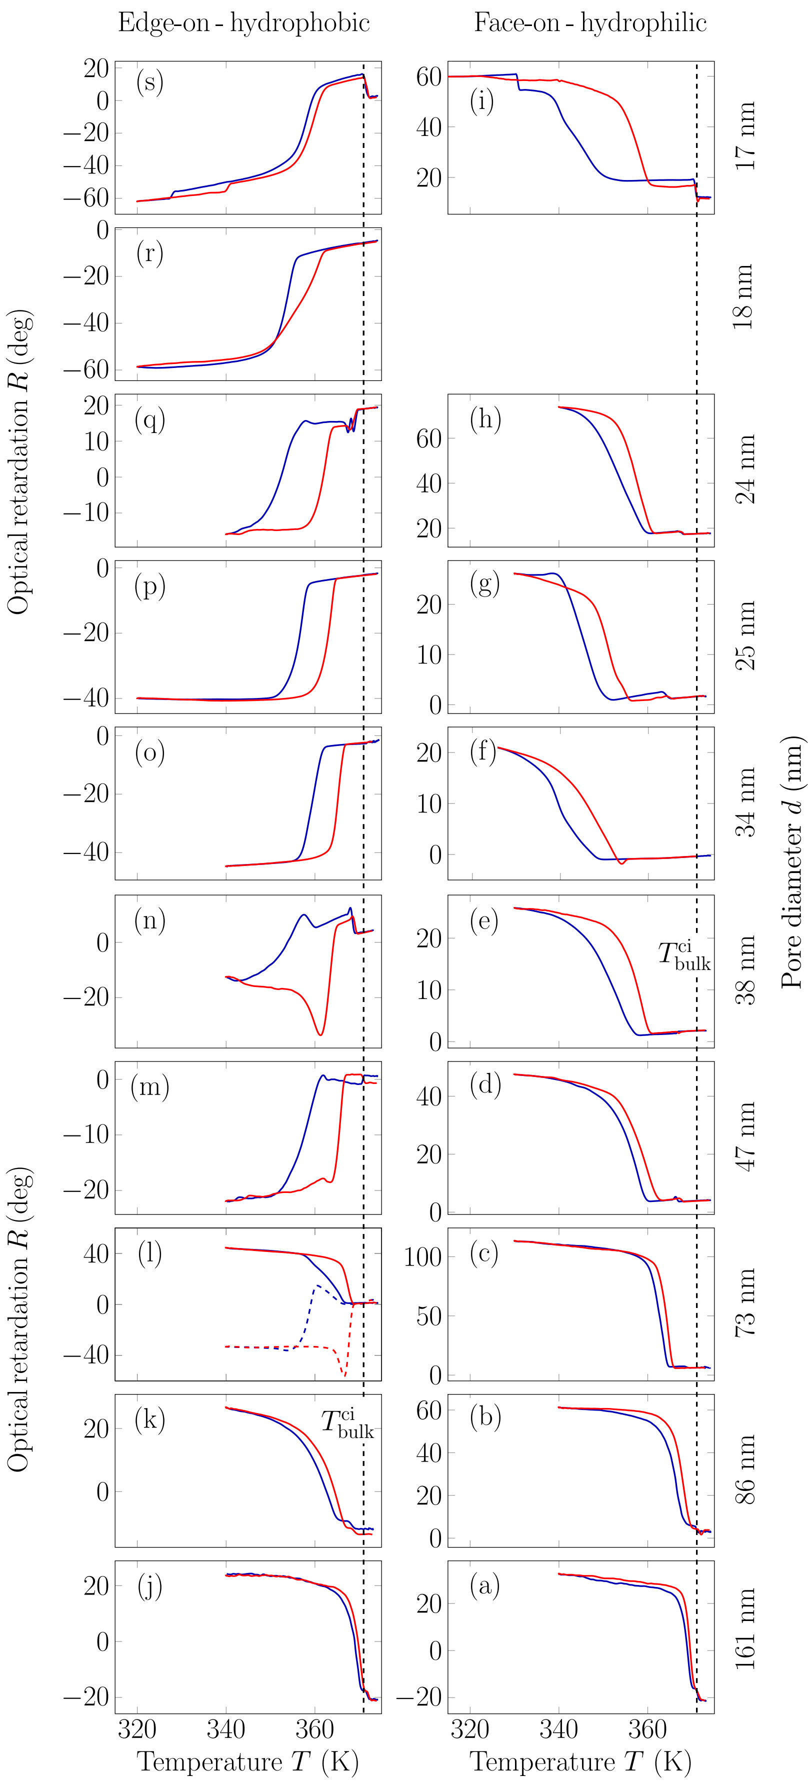


FIG. S3. Measured temperature depended optical retardation $R(T)$ of pore diameters from 17 nm to 161 nm in hydrophilic and hydrophobic AAO. Data is normalized by the thickness and porosity of corresponding AAO membrane, see Supplementary Tab. I.

## X-RAY DIFFRACTION

The transmission synchrotron X-ray diffraction experiment was performed at the P08 beamline of the PETRA III synchrotron (DESY) (beam size (VxH) = $(30\times100)\,\mu m^2$, $\lambda = 0.496$ Å, Perkin Elmer detector), the ID31 beamline of the European Synchrotron Radiation Facility (ESRF) (beam size (VxH) = $(100\times100)\,\mu m^2$, $\lambda = 0.1771$ Å, Pilatus3 XCdTe 2M detector) and the BM-11 (CMS) beamline at National Sychrotron Light Source (NSLS) II (beam size (VxH) = $(200\times200)\,\mu m^2$, $\lambda = 0.729$ Å, Pilatus3 XCdTe 2M detector) with temperatures in between $380-310$ K.

The discussion of the X-ray kinematics in the main text demonstrates that for the ideal situation that $k_i \perp \hat{p}$, i.e. $\omega$=90° particularly useful information can be gained in our scattering geometry with regard to the positional order in the $\hat{p}-\hat{\omega}$ plane, i.e. $(q_x - q_z)$ plane with $q_y$=0, see Fig. 4 of the main manuscript. However, for this configuration $k_i$ is parallel to the AAO membrane surface and thus the incident beam traverses the entire membrane cross-section, resulting in spurious x-ray intensities and absorption effects. Thus to confine in a maximal manner the wave vector transfers within planes aligned parallel to the pore axes, without however shadowing scattering directions in a $q$-range up to the intracolumnar order, $q_{dd}$ =$(1.726 \pm 0.008)$ Å$^{-1}$, the rotation angle $\omega$ in temperature scans was chosen as close as possible to 90°, i.e. $\omega = 85°$. Thereby, the wave vector transfers have still small contributions within planes aligned perpendicular to the $\hat{p}-\hat{\omega}$, i.e. in the $q_y$ direction. Note, however, that for the textures in our experiments the randomization about the long pore axis and the ring-like (100) Bragg intensity in reciprocal space mean that even for quite large deviations from $\chi$=90°, the Ewald sphere cuts in these ring-like structures, resulting in nearly six-fold diffraction patterns. This is particularly obvious from Fig. 4 of the main text. In the Results section of the main manuscript, these deviations are tacitly neglected in the qualitative discussions of the reciprocal space pictures. Most prominently the deviation from $\omega = 90°$ leads to a deviation of the streaks typical of the intracolumnar order from a perfect polar centering as can be seen in the movies M1 and M2 in the ESI by stopping the animations for $\hat{p}$ having an angle of about 85° with regard to the incident beam direction.

### A. Determination of domain sizes

Extracting from the diffraction patterns the full width at half maximum (FWHM), determined by performing Gaussian fits to the Bragg intensity curves derived by radial scans (fixed $\chi$ and variable $q$) and properly accounting for the instrumental broadening, as measured by a bulk reference powder, can be used to determine the average crystal or domain size $\xi$ in the direction of the radial scan. Employing the Scherrer equation $\xi = K\cdot\lambda/\Delta\theta\cdot\cos(\theta)$ with wavelength $\lambda$, Bragg angle $\theta$, FWHM expressed in degree $\Delta\theta$ and empirical proportionality factor $K = 0.9$, this has been done for reflections with $\chi$=0 or $\chi$=180 (parallel to $\hat{p}$) for the determination of the domain size along the long channel axis, i.e. the determination of $\xi_{\|}$ and for $\chi$=90 or $\chi$=270 (perpendicular to $\hat{p}$) for the determination of the domain size perpendicular to long pore axis, resulting in values for $\xi_{\perp}$, respectively. For those textures, where no Bragg reflection was parallel or perpendicular to $\hat{p}$, this procedure was applied to reflections close to the parallel or perpendicular direction, i.e. for $\chi$=30° and $\chi$=60° respectively. Then from this correlation length, the one in the perpendicular or parallel direction was calculated assuming that the measured one is just a projection of $\xi_{\perp}$ or $\xi_{\|}$. Note that such calculations can lead to apparent smaller domain sizes in the projections parallel to $\hat{p}$, because of the correlation length limits given by the finite size perpendicular to $\hat{p}$. However, the behaviour as a function of pore size gave no hints for such artefacts.

### B. X-ray intensity calculations for temperature scans

To semi-quantitatively analyse the temperature dependence of the texture formation intensities characteristic of the $(100)_{\|}$ and $(100)_{\perp}$ domains were calculated by summing up the Bragg intensities at $\chi_{\|}$ and $\chi_{\perp}$ values while integrating in sections with fixed cross-sections. The diffraction patterns for a fixed $\omega$=85 ° were used. For the distinct domains the corresponding reflections were selected and the intensity was integrated in equal quadratic regions. In general the diffraction spots at approx. $\chi$ = 30° for the parallel domain and approx. $\chi$ = 60°were chosen for the integration. Thereby the width in $\chi$ was selected so that the entire peak width was used for the integration. The $q$-range was chosen so that a Gauss fit could be performed sucessfully. As an example the selected integration values for diffraction pattern in Fig. 6(a)(iii) are given here: The $q$-range was chosen from 0.334 - 0.349 $Å^{-1}$. The width in $\chi$ around the azimuth angle of highest intensity was 10 degrees. No absorption or correlation lengths corrections were considered, since this analysis is aimed at a study of the appearance of the distinct domains as a function of temperature, particularly in comparison to the optical data, not at a full quantitative analysis. As outlined in the main manuscript distinct changes as a function

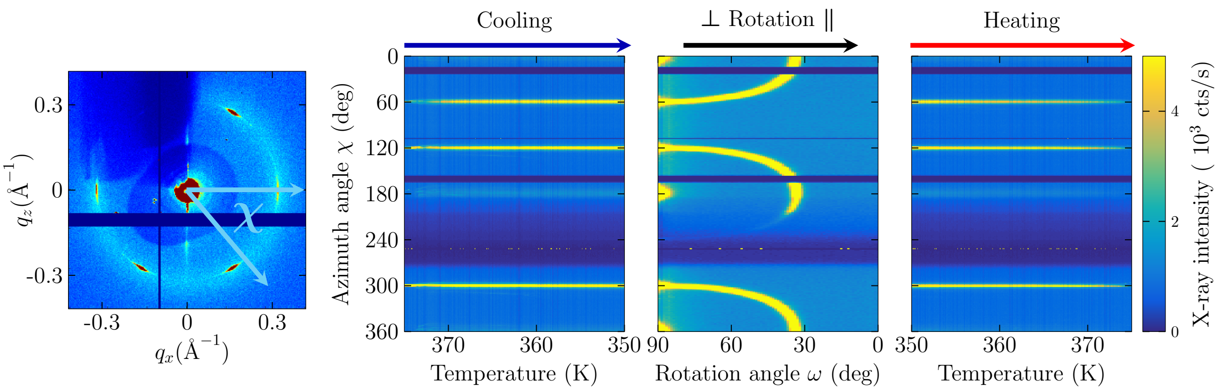


FIG. S4. Exemplary X-ray scattering data set of HAT6 in hydrophilic AAO with $d = 161\,\text{nm}$. (Left) Definition of azimuth angle $\chi$ as discussed in the text. (Right) Exemplary presentation of axis labelling for Bragg intensities shown in Figs. 5 and 7 of the main document. Plotted are intensities for a cooling ($\omega = 85°$), sample rotation ($\omega = 90° \rightarrow 0°$) and heating ($\omega = 85°$) scan extracted for each azimuth angle $\chi$.

of texture formation occur in our scattering geometry for a wavevector transfer $q_{(100)}$ in form of movements of Bragg peaks in azimuthal direction upon sample rotation. Therefore intensity scans in the azimuthal directions both as a function of temperature and as a function of sample rotation can be used for an efficient presentation of the structural evolutions upon cooling, rotation and heating. In those plots the intensity at $q_{(100)}$ is shown as a function of azimuthal angle $\chi$ (vertical axis) and sample rotation angle $\omega$ (horizontal axis) starting from a $\vec{k_i} \perp \hat{p}$ to $\vec{k_i} \parallel \hat{p}$ orientation, see Fig. S4 for an example of such a presentation.

## MONTE CARLO SIMULATIONS

Monte Carlo simulations of $N$ DLC molecules in the isothermal-isobaric ensemble expanded by temperature [3–7], employing the Gay-Berne-II model for the DLC [8–10] were performed.

To improve the equilibration of our simulated system, we use parallel tempering [4] and consider a set of reciprocal temperatures $\beta_m = 1/k_B T_m$, $m = 1, \ldots, N_R$, where $k_B$ is the Boltzmann constant and $T_m$ are temperatures, and use an expansion of the isothermal-isobaric ensemble (NPT) [5, 6]. This gives us a swapping probability between the configurations $x_m, x_{m+1}$ of two neighbouring temperatures $\beta_m, \beta_{m+1}$ of $p_{\text{acc}}(x_m \leftrightarrow x_{m+1}) = \exp\left[\Delta\beta(\Delta E + P\Delta V)\right]$.

We implemented the method for parallel simulation using up to $N_R = 96$ reciprocal temperatures $\beta_m$ running on different CPUs that communicate via Message Passing Interface (MPI). At each temperature a replica of the $N$ molecule system is simulated. At the start of each simulation, all replicas are initialised with a different random molecular configuration (positions and orientations). The simulation is carried out in the following manner: firstly, for each replica $(6N + 3)$ standard NPT Monte-Carlo steps are performed, secondly a replica exchange is attempted between a randomly selected pair of replicas with consecutive temperatures. After 500000 such steps, we start collecting ensemble averages. The main results of these simulations, in particular with regard to the circular concentric columnar state in cylindrical confinement have already been reported in Ref. [10]. Here, they were employed to achieve proper, physics-based visualisations of the distinct confined textures.


[1] A. V. Kityk, M. Wolff, K. Knorr, D. Morineau, R. Lefort, and P. Huber, Phys. Rev. Lett. **101**, 187801 (2008).
[2] A. V. Kityk, K. Knorr, and P. Huber, Phys. Rev. B **80**, 035421 (2009).
[3] D. Caprion, Eur. Phys. J. E **28**, 305 (2009).
[4] R. H. Swendsen and J.-S. Wang, Phys. Rev. Lett. **57**, 2607 (1986).
[5] Q. Yan and J. J. de Pablo, J. Chem. Phys. **111**, 9509 (1999).
[6] D. J. Earl and M. W. Deem, Phys. Chem. Chem. Phys. **7**, 3910 (2005).
[7] W. Lechner and C. Dellago, J. Chem. Phys. **129**, 114707 (2008).
[8] M. A. Bates and G. R. Luckhurst, J. Chem. Phys. **104**, 6696 (1996).
[9] D. Caprion, L. Bellier-Castella, and J.-P. Ryckaert, Phys. Rev. E **67**, 041703 (2003).
[10] K. Sentker, A. W. Zantop, M. Lippmann, T. Hofmann, O. H. Seeck, A. V. Kityk, A. Yildirim, A. Schoenhals, M. G. Mazza, and P. Huber, Phys. Rev. Lett. **120**, 67801 (2018).
